# Supplementary material for: Time-Dependent Density Matrix Renormalization Group Algorithms for Nearly Exact Absorption and Fluorescence Spectra of Molecular Aggregates at Both Zero and Finite Temperature
Source: arXiv:1806.07443 ancillary file (2018-10-12)
Supplement: Supplementary file 1 [file ephMPS-si.pdf]

# Supporting Information: Time Dependent Density Matrix Renormalization Group Algorithms for Nearly Exact Absorption and Fluorescence Spectra of Molecular Aggregates at Both Zero and Finite Temperature

Jiajun Ren,[†] Zhigang Shuai,[*,†] and Garnet Kin-Lic Chan[*,‡]

†*MOE Key Laboratory of Organic OptoElectronics and Molecular Engineering, Department of Chemistry, Tsinghua University, Beijing 100084, People's Republic of China*

‡*Division of Chemistry and Chemical Engineering, California Institute of Technology, Pasadena, California 91125, United States*

E-mail: zgshuai@tsinghua.edu.cn; gkc1000@gmail.com

## 1. Time step $\tau$ in the Runge-Kutta method

The error in TD-DMRG comes from two sources. One is the numerical method to approximate the time propagator, such as the RK methods used in this work. The other is from the wavefunction compression in MPS by the SVD. The latter is usually dominant, and leads to increased errors if the time step is too small in TD-DMRG.[S1] However, the time step cannot be too large either, as there is a stable region for the time step in RK methods, outside of

which the propagation will diverge. The propagator in RK4 is approximated as

$$e^{-iH\tau} \approx U = 1 + (-iH\tau) + \frac{(-iH\tau)^2}{2!} + \frac{(-iH\tau)^3}{3!} + \frac{(-iH\tau)^4}{4!} \tag{1}$$

The stability condition is $|U| \leq 1$. We define a function:

$$f(z) = 1 + z + \frac{z^2}{2!} + \frac{z^3}{3!} + \frac{z^4}{4!} \tag{2}$$

It can be shown that if the absolute maximal eigenvalue $e$ of $H$ fulfills $|f(-ie \cdot \tau)| \leq 1$, then $|f(-iH \cdot \tau)| \leq 1$. We plot $|f(z)|$ in the complex plane in Figure.S1. In our calculations, we only consider real time propagation and imaginary time propagation. The extreme stable points in the corresponding imaginary axis and real axis are 2.828 and $-2.785$. Thus the time step $\tau, \Delta\beta$ should fulfill $\tau \cdot e < 2.828$ in the real time propagation and $\Delta\beta \cdot e < 2.785$ in the imaginary time propagation.

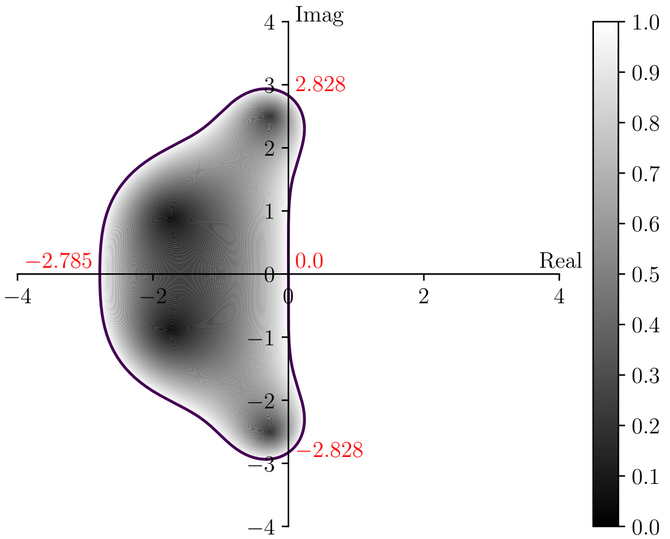


Figure S1: $|f(z)|$ in the complex plane. $|f(z)| = 1$ contour is plotted.

## 2. Error due to 4th-order Runge-Kutta integration

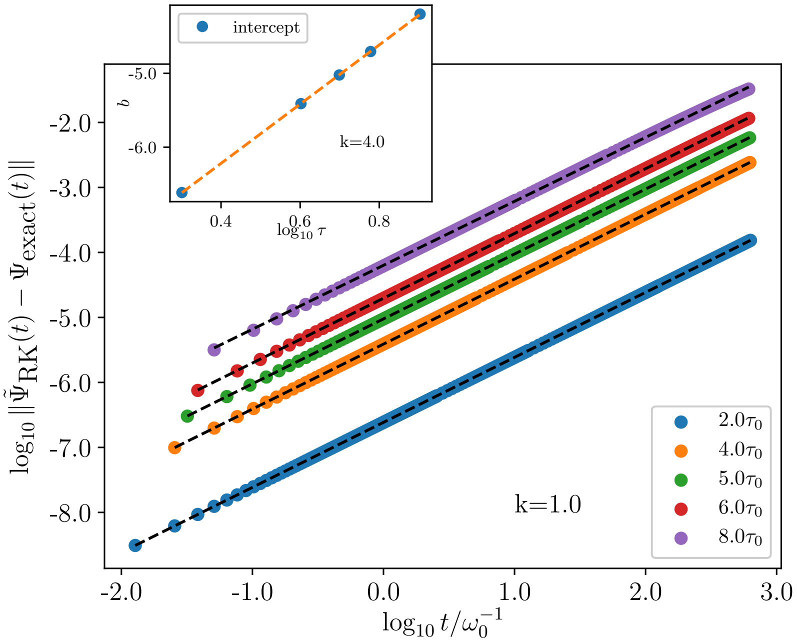


Figure S2: The wavefunction error $\|\Psi_{\mathrm{RK}}(t)-\Psi_{\mathrm{exact}}(t)\|$ versus time $t$ with different time steps $\tau$. $\tau_0 = 0.00639/\omega_0$.

To check the error due to the Runge-Kutta integration, we directly propagate the wavefunction in the full configuration interaction space with the 4th-order Runge-Kutta method. By a linear fit, we find that the relationship between the global error and the time is $O(t\tau^4)$, which is a well-known result in initial value problems (IVP) solved by RK4.

## 3. Chain representation vs. star representation

The chain mapping transformation maps the Holstein Hamiltonian from the star representation to the chain representation (see Figure S3).

The Hamiltonian in the star representation is:

$$\hat{H}_{\mathrm{star}} = \sum_i \varepsilon_i a_i^\dagger a_i + \sum_{ij} J_{ij} a_i^\dagger a_j + \sum_{in} \omega_{in} g_{in} a_i^\dagger a_i (b_{in}^\dagger + b_{in}) + \sum_{in} \omega_{in} b_{in}^\dagger b_{in} \tag{3}$$

After transformation, the Hamiltonian in the chain representation is:

$$\hat{H}_{\text{chain}} = \sum_i \varepsilon_i a_i^\dagger a_i + \sum_{ij} J_{ij} a_i^\dagger a_j + \sum_i V_{\text{tot,i}} a_i^\dagger a_i (\tilde{b}_{i0}^\dagger + \tilde{b}_{i0}) + \sum_{in} \alpha_{in} \tilde{b}_{in}^\dagger \tilde{b}_{in} + \sum_{in} \beta_{in} (\tilde{b}_{in}^\dagger \tilde{b}_{i,n-1} + h.c.) \tag{4}$$

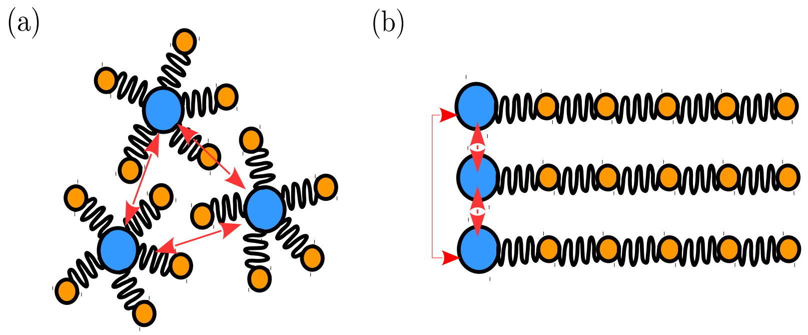


Figure S3: The interaction map of the Hamiltonian in the (a) star representation (b) chain representation.

The form of the electronic part of Hamiltonian in eq.(3) and eq.(4) is the same. The first vibrational site $\tilde{b}_{i0}$ in eq.(4) depends on all the original electron-phonon interaction terms as it is a linear combination of the original vibrational degrees of freedom. Since the transformation is carried out for each molecule separately, the molecular index $i$ is omitted.

$$\tilde{b}_0 = \frac{1}{V_{\text{tot}}} \sum_n g_n \omega_n b_n \tag{5}$$

$V_{\text{tot}}$ is the normalization factor.

$$V_{\text{tot}} = \sqrt{\sum_n (g_n \omega_n)^2} \tag{6}$$

The form of the vibrational Hamiltonian of each molecule in eq.(3) is $H_{\text{vib}} = \mathbf{B}^\dagger \mathbf{\Omega} \mathbf{B}$, where $\mathbf{B} = [b_1, b_2, \cdots, b_n]$, $\mathbf{\Omega} = \text{diag}(\omega_1, \omega_2, \cdots, \omega_n)$. To transform this into the chain

representation as in Figure S3(b), $\mathbf{\Omega}$ should be transformed into a tri-diagonal form $\mathbf{\Omega}'$ through a unitary rotation, $H_{\text{vib}} = \mathbf{B}^\dagger\mathbf{U}^\dagger\mathbf{\Omega}'\mathbf{U}\mathbf{B}$. In practice, the unitary matrix $\mathbf{U}$ can be obtained by the Lanczos algorithm, where the first vector in the unitary matrix $\mathbf{U}$ is fixed to be $|v_0\rangle = \frac{1}{V_{\text{tot}}}[g_0\omega_0, \cdots, g_n\omega_n]$ in eq.(5).

Based on this initial vector, the Krylov space can be constructed by the recurrence relation,

$$\beta_{n+1}|v_{n+1}\rangle = |\tilde{v}_{n+1}\rangle = \hat{H}|v_n\rangle - \alpha_n|v_n\rangle - \beta_n|v_{n-1}\rangle \tag{7}$$

$$\alpha_n = \langle v_n|\hat{H}|v_n\rangle \tag{8}$$

$$\beta_n^2 = \langle \tilde{v}_n|\tilde{v}_n\rangle, \beta_0 = 0 \tag{9}$$

Then, $\alpha_n$ and $\beta_n$ are the parameters in eq.(4).

After this transformation, the interaction in the Hamiltonian is of nearest neighbor form, except for the excitonic coupling. It is sometimes argued that DMRG is more efficient for nearest neighbor interaction. However, recent studies show that the opposite is true in impurity models.[S2] We have also compared these two representations when calculating the zero temperature absorption spectrum of the J-type PBI dimer. (See Figure.S4) The accuracy is very similar in both cases with the same SVD threshold, but the virtual bond dimension of the MPS in the chain representation grows faster than when in the star representation. Therefore, the star representation is preferred for long time propagations. A further drawback of the chain representation is that the locality of the Hamiltonian in the zero-exciton space is lost, so the zero temperature fluorescence requires a full TD-DMRG propagation.

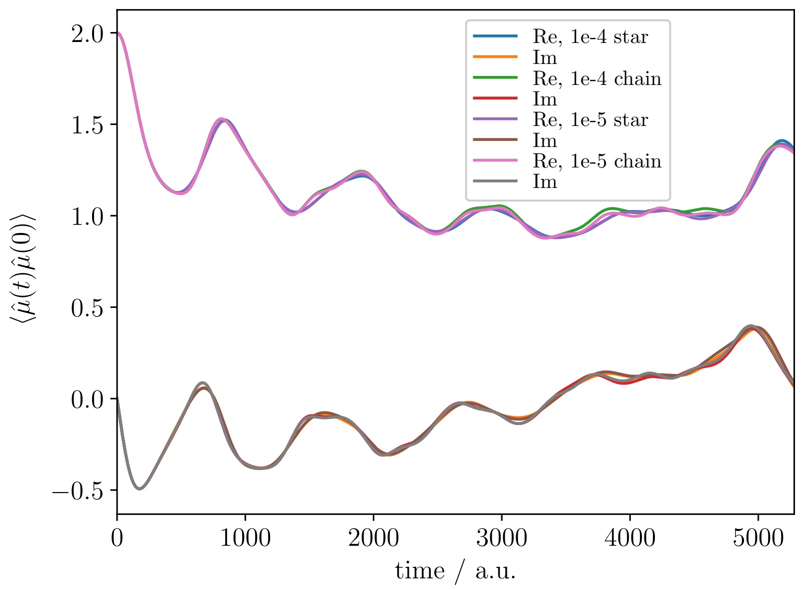


(a)

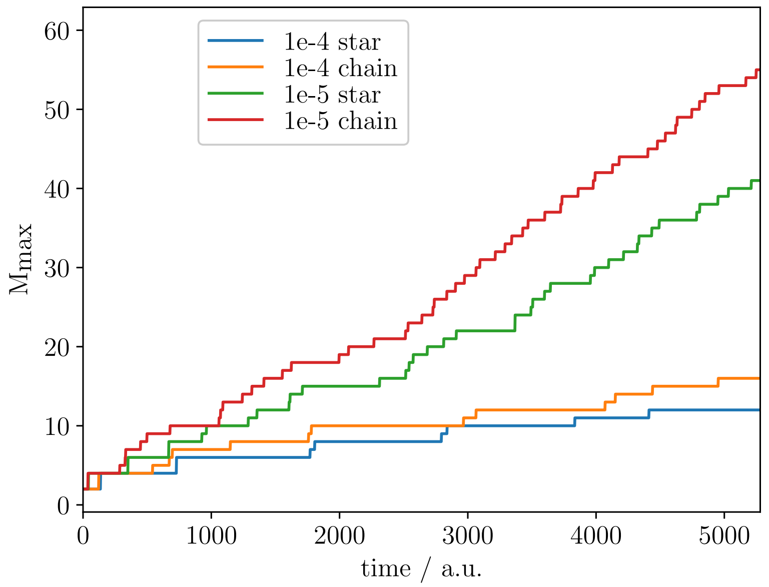


(b)

Figure S4: (a) dipole-dipole time correlation function (b) maximal virtual bond dimension of MPS in the star representation and chain representation calculation, with time step $\tau = 1$ a.u, total steps $N = 5200$, SVD cutoff $10^{-4}$ and $10^{-5}$.

# 4. Quantum chemistry parameters for the DSB crystal

The parameters of the exciton-exciton coupling and exciton-phonon coupling are adopted from Ref. S3. The selected normal modes with the largest 14 Huang-Rhys factors (>0.02) are listed in Table.S1. The exciton-exciton coupling in the DSB dimer can be directly found in the SI of Ref. S3.

Table S1: The selected normal modes and the corresponding Huang-Rhys factors

| index | frequency / $cm^{-1}$ | Huang-Rhys factor S |
|---|---|---|
| 1 | 154.22 | 0.41897 |
| 2 | 1658.65 | 0.30658 |
| 3 | 1706.77 | 0.13216 |
| 4 | 1219.84 | 0.12597 |
| 5 | 1385.15 | 0.08927 |
| 6 | 1608.48 | 0.06161 |
| 7 | 322.88 | 0.04534 |
| 8 | 1231.41 | 0.03764 |
| 9 | 907.14 | 0.03273 |
| 10 | 1672.04 | 0.02984 |
| 11 | 671.67 | 0.02663 |
| 12 | 140.53 | 0.02268 |
| 13 | 1249.46 | 0.02176 |
| 14 | 132.8 | 0.02158 |

# References


(S1) Gobert, D.; Kollath, C.; Schollwöck, U.; Schütz, G. Real-time dynamics in spin-1 2 chains with adaptive time-dependent density matrix renormalization group. *Phys. Rev. E* **2005**, *71*, 036102.

(S2) Wolf, F. A.; McCulloch, I. P.; Schollwöck, U. Solving oonequilibrium dynamical mean-field theory using matrix product states. *Phys. Rev. B* **2014**, *90*, 235131.

(S3) Wenqiang, L.; Qian, P.; Yujun, X.; Tian, Z.; Zhigang, S. Effect of intermolecular

excited-state interaction on vibrationally resolved optical spectra in organic molecular aggregates. *Acta Chim. Sin.* **2016**, *74*, 902–909.
